# Supplementary material for: Polestar: Drift-Aware Cache Calibration and Token Commitment for Efficient Inference of Diffusion LLMs
Source: arXiv:2607.14107 source file (2026-05-07)
Supplement: Supplementary file 1 [file results.tex]

% \input{tables/main_results_appendix}
% \input{tables/llada_v_appendix}
% \input{tables/parallel_bench_hard}
